# Supplementary material for: Optimal operation of hole spin qubits
Source: arXiv:2412.13069 source file (2024-12-17)

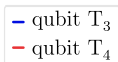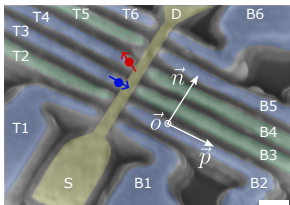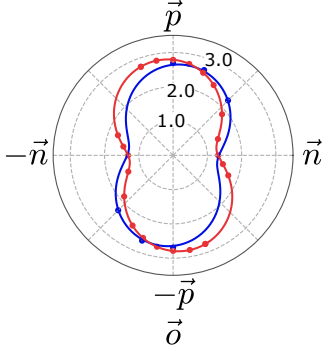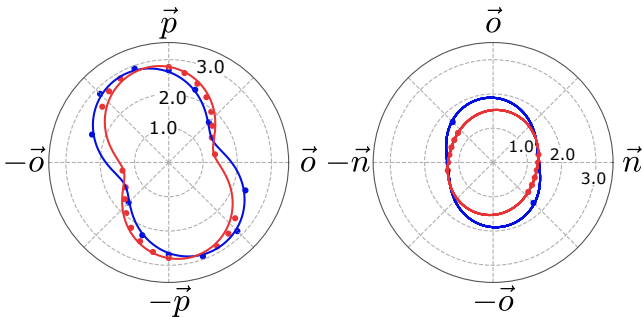

Supplement: Supplementary file 1 [file 1_comparison_g_qubits.pdf]
