# Supplementary material for: Optimal operation of hole spin qubits
Source: arXiv:2412.13069 source file (2024-12-17)

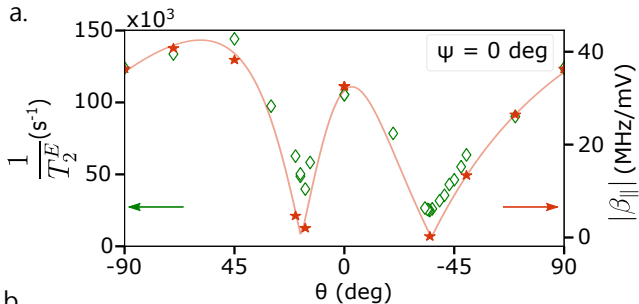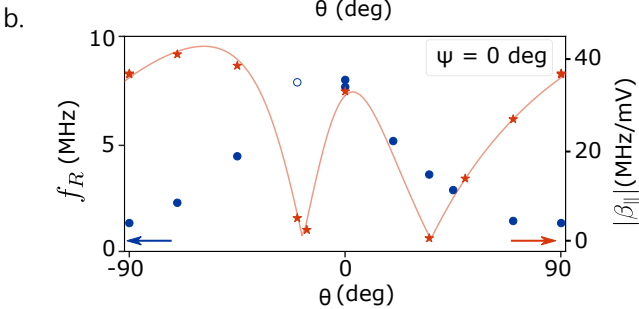

Supplement: Supplementary file 2 [file 3_Rabi_n_Echo_vs_angle.pdf]
